# Supplementary material for: A Fast Insertion Operator for Ridesharing over Time-Dependent Road Networks
Source: arXiv:2303.03614 source file (2023-03-07)
Supplement: Supplementary file 1 [file 08_appendix.tex]

% \vspace{-2ex}
\zeng{
\section{Appendix of Missing Proofs}

% \vspace{-1ex}
\subsection{Proof of \lemref{lem:divide-approx}}\label{app:lem:divide-approx}
\begin{proof}
	To prove this theorem, we only need to show the distortion guarantee of \algoref{alg:construct} is $O(\log{n})$,
	since it has been shown $O(\log{n})$ is a tight bound for tree embeddings \cite{DBLP:conf/focs/Bartal96,hststoc03}.

	We present the following proof by \textit{mathematical induction} based on the approximation result from \cite{hststoc03},
	since Fakcharoenphol \etal \cite{hststoc03} has proved that the HST constructed by their algorithm (denoted by \FRT)  has a distortion guarantee of $O(\log{n})$.
	As their proof assumes that $\Dis(x,y) \ge 1$ for any different objects $x \neq y$ (\eg by normalization), we also assume the function $\Dis(,)$ has been normalized (in the proof only).
	We also assume both methods are given the same parameter $\beta$, since the distribution of $\beta$ is the same.
	Based on these settings, we have the distance functions for both methods are $\Dis_{\T}(u,v) = \frac{1}{root.\distort} \sum_{e \in path(u,v)}{\EW(e)}$,
	where $u,v$ are two leaves, $path(u,v)$ denotes the tree path from $u$ to $v$,
	and $\EW(e)$ denotes the edge weight of the edge $e$.
	
	When there are only one object in the metric $\MS$, either \algoref{alg:construct} or \FRT will construct the same tree (\ie a single root).
	
	When there are more than one object, we assume $O(\log{n})$ holds for $n = m$ and prove it also holds for $n = m+1$.
	Specifically, we use $\cp_1$ to denote the first center sampled by \algoref{alg:construct} in line 5.
	Then, at any level $i=2,\cdots,\HT+1$, the number of remaining objects in $\V_{i-1} \setminus \V_{i}$ is no more than $n-1=m+1-1=m$,
	since a leaf will eventually represent the object $\cp$, \ie $\Leaf(\cp_1)$.
	It indicates that the distortion guarantees of subtrees, which are subsequently constructed based on the remaining objects,
	are all bounded by $O(\log{m}) = O(\log{n})$.
	It still remains to be proved that $\E_{\cp_1}[\Dis_{\T}(\Leaf(x),\Leaf(\cp_1))] \ge \frac{1}{\rho} \cdot \Dis(x,\cp_1)$,
	where the distortion $\rho = 96\ln{n} = O(\log{n})$.
	
	This statement is true, because the centers of \FRT \cite{hststoc03} are picked from a random permutation $\pi$ of the objects $\V$.
	Thus, its first center (say $\cp_1'$) is also uniformly sampled from $\V$.
	In other words, $\cp_1$ has the same distribution as the first center $\cp_1'$ in \FRT.
	Since \FRT has proved that $\E_{\cp_1'}[\Dis_{\T}(\Leaf(x),\Leaf(\cp_1))] \ge \frac{1}{96\ln{n}} \cdot \Dis(x,\cp_1')$ (see the proof in Sec. 2.3 \cite{hststoc03}),
	we complete our proof.
\end{proof}

% \vspace{-2ex}
\subsection{Proof of \lemref{lem:range-prune-node}}\label{app:range-prune-node}
\begin{proof}
	Let $x$ be an object contained in $v$ and $y$ be an object contained in its child node $u$.
	Based on the node structure and construction algorithm,
	we know $\Dis(v.\cp, x) \le \radat(v.\level)$, $\Dis(v.\cp, y) \le \radat(v.\level)$, $\Dis(u.\cp, y) \le \radat(u.\level)$, and $u.\discp = \Dis(v.\cp, u.\cp)$.
	
	\textbf{Case (1)}. We derive the \textit{upper bound} of $\Dis(q,x)$ as
	\begin{equation*}
		\Dis(q,x) \le \Dis(v.\cp,q) + \Dis(v.\cp. x) \le \distoq + \radat(v.\level).
	\end{equation*}
	The prerequisite of this case is $\distoq + \radat(v.\level) \le r$,
	which means $\Dis(q,x) \le r$ and $x$ is within the query range.
	
	\textbf{Case (2)}. $LB$ and $UB$ denote the lower bound and upper bound of distances between $v.\cp$ and any object $z$ (if possible) which is in the query range and contained in $v$.
	As $z$ is in the query range, we know $\Dis(q,z) \le r$.
	By triangle inequality, we have $\Dis(v.\cp,z) \ge \Dis(v.\cp,q) - \Dis(q,z) \ge \distoq - r$ and $\Dis(v.\cp,z) \le \Dis(v.\cp,q) + \Dis(q,z) \le \distoq + r$.
	Since $z$ is contained in $v$, we know $\Dis(v.\cp,z) \le \radat(v.\level)$.
	Now, we have proved the correctness of $LB$ and $UB$.
	We next derive the \textit{lower bound} of $\Dis(q,x)$ as
	\begin{equation*}
		\Dis(q,x) \ge \Dis(v.\cp,q) - \Dis(v.\cp. x) \ge \distoq - \radat(v.\level).
	\end{equation*}
	The prerequisite of this case is $\radat(v.\level) < LB < \distoq-r$, which means $\Dis(q,x) > r$ and $x$ is not in the query range.
	
	\textbf{Case (3)}. We derive the \textit{upper bound} of the distance $\Dis(q, y)$ as: 
	\begin{align*}
		\Dis(q, y) &\le \Dis(q, v.\cp) + \Dis(v.\cp, y)  \le \distoq + \radat(v.\level) \\
		\Dis(q, y) &\le \Dis(q, v.\cp) + \Dis(v.\cp, u.\cp) + \Dis(u.\cp, y)  \\
			&\le  \distoq + u.\discp + \radat(u.\level)
	\end{align*}
	The prerequisite of this case is $\distoq + \radat(v.\level) \le r$ and $\distoq + u.\discp+\radat(u.\level) \le r$, 
	which means $\Dis(q,y) \le r$ and $y$ is within the query range.
	
	\textbf{Case (4)}. $lb$ and $ub$ denote the lower bound and upper bound of distance between $v.\cp$ and $y$.
	We first prove the correctness of $lb$.
	As $u$ contains $y$ and $u$ is not $v$'s left-most child, we can derive $\Dis(v.\cp,y) > \radat(v.\level+1)$ (Otherwise, the left-most child will contain $y$).
	Since $v$ is the lowest common ancestor of the singleton leaves of $v.\cp$ and $y$,
	we have $\DisT(y,v.\cp) = \DisTAt(v.\level)$ based on \defref{def:tree-embedding}. 
	Based on \defref{def:embedding},
	we know $\Dis(y,v.\cp) \ge \DisT(y,v.\cp)/v.\distort \ge \DisTAt(v.\level)/v.\distort$.
	By triangle inequality, we have
	$\Dis(y,v.\cp) \ge \Dis(v.\cp,u.\cp) - \Dis(y,u.\cp) \ge u.\discp-\radat(u.\level)$.
	
	We next prove the correctness of $ub$.
	Similar to that of $lb$, we have
	$\Dis(y,v.\cp) \le \Dis(v.\cp,u.\cp) + \Dis(y,u.\cp) \ge u.\discp+\radat(u.\level)$.
	Since $v$ contains $y$, $\Dis(y,v.\cp) \le \radat(v.\level)$.
	
	We finally prove the statement of the fourth case.
	The prerequisite of this case is that $\ring(v.\cp, LB, UB)$ does not overlap with $\ring(v.\cp, lb, ub)$.
	Due to the definitions of these lower/upper bounds, the object $y$ cannot be in the query range,
	
	\textbf{Case (5)}. This case is a corollary of the second case.
	Let $v'$ be the left-most child node of $v$.
	Based on the construction algorithm, we know $\radat(v'.\level) \le \radat(v.\level+1)$ and $v'.\cp = v.\cp \implies \distoq' = \Dis(v'.\cp,q) = \distoq$.
	The prerequisite of this case is $\radat(v.\level+1) < LB$, where $LB = \max\{0, \distoq-r\}$.
	Thus, we have $\radat(v'.\level) < \max\{0, \distoq'-r\}$.
	We complete the proof by substituting $v',\distoq'$ for $v,\distoq$ in the second case.
	
	\textbf{Case (6)}. This case is a corollary of the fourth case.
	Based on the prerequisite, we can infer that $u2vLB \ge \radat(v.\level+1) > UB$.
	Thus, $\overlap(v.\cp, LB, UB, u2vLB, u2vUB)$ is always false.
\end{proof}

% \vspace{-2ex}
\subsection{Proof of \lemref{lem:range-prune-child-node}}\label{app:range-prune-child-node}
\begin{proof}
	Let $x$ be an object contained in $u_i$.
	Based on the node structure and construction algorithm,
	we know $\Dis(v.\cp, u^*.\cp) \le \radat(v.\level)$, $\Dis(v.\cp, x) \le \radat(v.\level)$, 
	$\Dis(u_i.\cp, x) \le \radat(u_i.\level)$, $u^*.\discp = \Dis(v.\cp, u^*.\cp)$, $u_i.\discp = \Dis(v.\cp, u_i.\cp)$.
	
	\textbf{Case (1)}.
	$LB$ and $UB$ denote the lower bound and upper bound of distances between $u^*.\cp$ and any object $z$ which is in the query range and contained in $u^*$.
	$lb$ and $ub$ denote the lower bound and upper bound of distance between $u^*.\cp$ and $x$.
	The proof of \lemref{lem:range-prune-node} (2) has shown the correctness of $LB$ and $\Dis(u^*.\cp,z) \le \distoq^*+r$.
	Hence, we only need to prove $\Dis(u^*.\cp,z) \le 2\radat(v.\level)$.
	As both $u^*.\cp$ and $z$ are contained in $v$, we know $\Dis(v.\cp, u^*.\cp) \le \radat(v.\level)$ and $\Dis(v.\cp, z) \le \radat(v.\level)$.
	By triangle inequality, we have $\Dis(v.\cp, u^*.\cp) + \Dis(v.\cp, z) \le \radat(v.\level) + \radat(v.\level)$.
	
	We next prove the correctness of $lb$.
	From the proof of \lemref{lem:range-prune-node} (4), we know $\Dis(u^*.\cp,x)$ is no smaller than $\radat(v.\level+1)$ and $\DisTAt(v.\level)/v.\distort$.
	By triangle inequality, we have
	$\Dis(u^*.\cp,x) \ge \Dis(u^*.\cp,u_i.\cp) - \Dis(u_i.\cp,x) \ge |\Dis(v.\cp,u^*.\cp) - \Dis(v.\cp,u_i.\cp)| - \radat(u_i.\level) \ge |u^*.\discp-u_i.\discp|-\radat(u_i.\level)$.
	
	Then, we prove the correctness of $ub$.
	From the proof of \lemref{lem:range-prune-node} (4), we know $\Dis(u^*.\cp,x) \le u^*.\discp + \radat(v.\level)$.
	Similar to the proof of $lb$, we can derive that
	$\Dis(u^*.\cp,x) \le \Dis(v.\cp,u^*.\cp) + \Dis(v.\cp,u_i.\cp) + \radat(u_i.\level) \le u^*.\discp+u_i.\discp+\radat(u_i.\level)$.
	
	We finally prove the statement of this case.
	If $\ring(u^*.\cp, LB, UB)$ does not overlap with $\ring(u^*.\cp, lb, ub)$.
	the object $x$ cannot be in the query range due to definitions of these bounds.
	
	\textbf{Case (2)}. The prerequisite of this case is $\max\{\radat(v.\level+1), \DisTAt(v.\level)/v.\distort\} > r + \distoq^*$, and this case is a corollary of the first case.
	\WLOG, let $y$ be an object contained in child nodes $u_i,\cdots,u_k$.
	Based on $lb$'s definition, we know $lb \ge \max\{\radat(v.\level+1), \DisTAt(v.\level)/v.\distort\}$ for any of these child nodes.
	Based on $UB$'s definition, we know $UB \ge \distoq^*+r$.
	Based on the prerequisite, we can infer $lb > UB$,
	which means $\overlap(u^*.\cp, LB, UB, lb, ub)$ is always false for these child nodes.
	Thus, $u_i$-$u_k$ can be pruned.
\end{proof}

% \vspace{-2ex}
\subsection{Proof of \lemref{lem:knn-prune-sibling}}\label{app:lem:knn-prune-sibling}
\begin{proof}
	Let $x$ be an object contained in $u_1$ and $y$ be an object contained in $v_2$-$v_k$.
	Based on the node structure and construction algorithm,	
	we know $p.\cp = v_1.\cp = u_1.\cp$, $\Dis(p.\cp,x) = \Dis(u_1.\cp,x) \le \radat(u_1.\level)$,
	$\Dis(p.\cp,y) = \Dis(v_1.\cp,y) \in (\radat(v_1.\level+1), \radat(v_1.\level)]$.
	Based on the definition of $\radat(\cdot)$, we know $\radat(v_1.\level) \ge \HSTk\radat(u_1.\level) \ge \HSTk^2\radat(u_1.\level+1)$.
	
	We first derive the lower bound of $\Dis(q,y)$ as follows.
	\begin{align*}
		\Dis(q,y) &\ge \Dis(p.\cp,y) - \Dis(p.\cp,q) \ge \Dis(p.\cp,y) - \distoq \\
			&> \radat(v_1.\level+1) - \radat(u_1.\level+1) \\
			&> \HSTk^2\radat(u_1.\level+1) - \radat(u_1.\level+1) \\
			&> 3\radat(u_1.\level+1)
	\end{align*}
	
	We next derive the upper bound of $\Dis(q,x)$ as follows.
	\begin{align*}
		\Dis(q,x) &\le \Dis(p.\cp,x) + \Dis(p.\cp,q) \le \Dis(p.\cp,x) + \distoq \\
			&\le \radat(u_1.\level) + \radat(u_1.\level+1) \\
			&\le \HSTk\radat(u_1.\level+1) + \radat(u_1.\level+1) \\
			&\le 3\radat(u_1.\level+1)
	\end{align*}
	
	Based on the prerequisite, $u_1$ contains at least $k$ objects (\eg $x$).
	The proof above indicates the their distances to $q$ are no larger than $3\radat(u_1.\level+1)$.
	Thus, the distance between $q$ and its $k$th nearest neighbor is at most $3\radat(u_1.\level+1)$.
	Since $\Dis(q,y) > 3\radat(u_1.\level+1)$, the object $y$ cannot be the k nearest neighbors of $q$ and hence can be pruned.
\end{proof}

% \vspace{-2ex}
\subsection{Proof of \lemref{lem:learn-estimate}}\label{app:lem:learn-estimate}
\begin{proof}
	Let $r$ be the $k$th nearest distance to the query object $q$
	and $\V'$ be the objects covered by the current node $v$ in line 4 of \algoref{alg:knn-estimate}.
	We can derive $r \le \max_{x \in \V'}{\Dis(q,x)}$.
	Thus, for any object $x \in \V'$, we have $\Dis(v.\cp,x) \le \radat(v.\level)$ due the construction of Lite-HST in \algoref{alg:construct}.
	By the triangle inequality, we know 
	\begin{equation*}
		\Dis(q,x) \le \Dis(q,v.\cp) + \Dis(v.\cp,x) \le \Dis(v.\cp,q) + \radat(v.\level)
	\end{equation*}
	Finally, since $\max_{x \in \V'}{\Dis(q,x)} \ge r$, we can simply derive that $\Dis(v.\cp,q) + \radat(v.\level) \ge r$, 
	which completes our proof.
\end{proof}
}
